# Supplementary material for: Visualizing the loss landscape of Self-supervised Vision Transformer
Source: arXiv:2405.18042 source file (2024-05-28)
Supplement: Supplementary file 1 [file appendix.tex]

\appendix

\begin{figure*}[t!]
\begin{center}
\scalebox{1.0}{
\includegraphics[width=1.\textwidth]{fig/epoch.pdf}
}
\end{center}
\caption{
\textbf{Loss landscapes of self-supervised vision transformer by MAE~\cite{he2022mae} and RC-MAE~\cite{lee2023rcmae} at different training epochs}. 
Note that as the learning progresses, the optimal point gets sharper.
}
% \vspace{-0.5cm}
\label{fig:epoch}
\end{figure*}
\section{Appendix}

Similar to~\Cref{fig:mae_epoch}, we visualize and compare loss landscapes of RC-MAE with MAE at different epochs as shown in~\Cref{fig:epoch}.
